# Supplementary material for: BrainNNExplainer: An Interpretable Graph Neural Network Framework for Brain Network based Disease Analysis
Source: arXiv:2107.05097 source file (2021-07-11)
Supplement: Supplementary file 1 [file appendix.tex]

\section{Node Index and Abbr of Atlas AAL90}

% Please add the following required packages to your document preamble:
% \usepackage{multirow}
% Please add the following required packages to your document preamble:
% \usepackage{multirow}
% Please add the following required packages to your document preamble:
% \usepackage{multirow}
\begin{table}[!htb]
\centering
\caption{The abbreviations of AAL regions}
\scriptsize
\begin{tabular}{|l|l|l|}
\hline
Index                 & Region                                                     & Abbr  \\ \hline
1, 2                  & Precental gyrus                                            & PG    \\ \hline
\multirow{8}{*}{3, 4} & \multirow{5}{*}{Superior frontal gyrus,   dorsolateral}    & DSFG  \\ \cline{3-3} 
                      &                                                            & OSFG  \\ \cline{3-3} 
                      &                                                            & MFG   \\ \cline{3-3} 
                      &                                                            & OMFG  \\ \cline{3-3} 
                      &                                                            & OPIFG \\ \cline{2-3} 
                      & \multirow{2}{*}{Inferior frontal gyrus,   triangular part} & TIFG  \\ \cline{3-3} 
                      &                                                            & OIFG  \\ \cline{2-3} 
                      & Rolandic operculum                                         & RO    \\ \hline
19, 20                & Supplementary motor area                                   & SMA   \\ \hline
21,22                 & Olfactory cortex                                           & OC    \\ \hline
23, 24                & Superior frontal gyrus,   medial                           & MSFG  \\ \hline
25, 26                & Superior frontal gyrus,   medial orbital                   & MOSFG \\ \hline
27, 28                & Gyrus rectus                                               & GR    \\ \hline
29, 30                & Insula                                                     & INS   \\ \hline
31, 32                & Anterior cingulate and   paracingulate gyri                & ACC   \\ \hline
33, 34                & Median cingulate and paracingulate   gyri                  & MCPG  \\ \hline
35, 36                & Posterior cingulate gyrus                                  & PCC   \\ \hline
37, 38                & Hippocampus                                                & HIP   \\ \hline
39, 40                & Parahippocampal gyrus                                      & PHG   \\ \hline
41, 42                & Amygdala                                                   & AMY   \\ \hline
43, 44                & Calcarine fissure and   surrounding cortex2                & CF    \\ \hline
45, 46                & Cuneus                                                     & CUN   \\ \hline
47, 48                & Lingual gyrus                                              & LG    \\ \hline
49, 50                & Superior occipital gyrus                                   & SOG   \\ \hline
51, 52                & Middle occipital gyrus                                     & MOG   \\ \hline
53, 54                & Inferior occipital gyrus                                   & IOG   \\ \hline
55, 56                & Fusiform gyrus                                             & FG    \\ \hline
57, 58                & Postcentral gyrus                                          & POG   \\ \hline
59, 60                & Superior parietal gyrus                                    & SPG   \\ \hline
61, 62                & Inferior parietal, but   supramarginal and angular gyri    & SMAG  \\ \hline
63, 64                & Supramarginal gyrus                                        & SMG   \\ \hline
65, 66                & Angular gyrus                                              & AG    \\ \hline
67, 68                & Precuneus                                                  & PRE   \\ \hline
69, 70                & Paracentral lobule                                         & PL    \\ \hline
71, 72                & Caudate nucleus                                            & CN    \\ \hline
73, 74                & Lenticular nucleus, putamen                                & PUT   \\ \hline
75, 76                & Lenticular nucleus,   pallidum                             & PAL   \\ \hline
77, 78                & Thalamus                                                   & THA   \\ \hline
79, 80                & Heschl gyrus                                               & HG    \\ \hline
81, 82                & Superior temporal gyrus                                    & STG   \\ \hline
83, 84                & Temporal pole: superior   temporal gyrus                   & TSTG  \\ \hline
85, 86                & Middle temporal gyrus                                      & MTG   \\ \hline
87, 88                & Temporal pole: middle   temporal gyrus                     & TMTG  \\ \hline
89, 90                & Inferior temporal gyrus                                    & ITG   \\ \hline
\end{tabular}
\end{table}

% The table shows the abbreviations of AAL regions except the cerebellum \cite{chen2021decreased}, which can be summarized as Visual = (43-56, 59, 60, 89, 90); Auditory = (17, 18, 79-82); Bilateral Limbic = (21, 22, 27, 28, 37-42, 83, 84, 87, 88); Default Mode Network (DMN) = (3, 4, 5, 6, 9, 10, 23-26, 31, 32, 33, 34, 35, 36, 65-68); Sensorimotor = (1, 2, 19, 20, 57, 58, 69, 70); Subcortical = (71-78); Memory = (85, 86, 89, 90); Cognitive control = (7, 8 , 11-16, 29, 30, 61, 62, 63, 64).
